# Supplementary material for: Does Label Differential Privacy Prevent Label Inference Attacks?
Source: arXiv:2202.12968 source file (2023-06-03)
Supplement: Supplementary file 1 [file appendix_data_reconstruction.tex]

\section{Data Reconstruction Attack}
\paragraph{Data assumption.}
We have assumption for the data.
\begin{assumption}
We assume training data $(X_i, \by_i)$ is i.i.d. sampled from an underlying distribution $\calD$ on the domain of $\calZ$.
\end{assumption}

\paragraph{Threat model.} 
\begin{itemize}
    \item The adversary has the full knowledge of the released item, e.g. the model or the gradient in FL, $f := \calA^{\rm tr}(X, \by)$, where $\calA^{\rm tr}$ is the algorithm, because $f$ is targeted item to be released publicly.
    \item (optional) The adversary has the prior of data distribution $\calD$. It is similar to the setting of membership inference attack \cite{yeom2018privacy}. 
\end{itemize}
The attacker tries to infer $\bz_i=(X_i, \by_i)$. We define $\calA^{\rm att}$ as the attack algorithm taking $f$ (and $\calD$) as input and outputs an estimator of $\hat{\bz}_i$ in the domain $\calZ$.

\paragraph{Excess advantage.} 
We can define the advantage as
\begin{equation}
    {\rm \text{Adv}}(\calA^{\rm att}, (f, \calD)) = \bbE\left[g(\hat{\bz}_i, \bz_i )\right],
\end{equation}
where $g:\calZ\to\calZ$ is the benefit function and the randomness comes from the data generation, training process and the possible attack process. We have following assumption for $g$, out of representation simplicity. The results could be generalized to any $g$ that is bounded.
\begin{assumption}
$\forall \hat{\bz}_i, \bz_i\in \calZ, g(\hat{\bz}_i, \bz_i )\in [0, 1]$
\end{assumption}
Then we could define the excess advantage as 
\begin{align}
    {\rm \text{Exc-Adv}}\left(\calA^{\rm att}, \calK\right) &:= {\rm \text{Adv}}\left(\calA^{\rm att}, \calK\right) \nonumber\\
    &- \max_{z\in \calZ}\bbE_{\bz_i} \left[g(z, \bz_i)\right].
\end{align}
To understand the base, consider a special case that $\calZ \in[0, 1]^{d+1}$ and $g(\hat{\bz}_i, \bz_i):=1 - \frac{1}{d+1}\sum_{j=1}^{d+1}(\hat{\bz}_i^j- \bz_i^j)^2\in [0, 1]$ is the mean squared error. We could check that $g(\hat{\bz}_i, \bz_i )\in[0, 1]$. Moreover, the base is actually $1-Var(\bz_i)/(d+1)$, which is $1$ minus the normalized variance of the data.

We then have following theorem:
\begin{theorem}
With Assumption 1 and 2, if $f$ is $(\varepsilon, \delta)$-differentially private,
$$
{\rm \text{Exc-Adv}}\left(\calA^{\rm att}, \calK\right)\leq (1 - e^{-\varepsilon}) + \delta|\calZ|,
$$ 
where $|\calZ|$ is the size of $|\calZ|$ when $\calZ$ is a discrete space, or $|\calZ| = \int_{z\in\calZ}1\diff z$ when $\calZ$ is a continuous space.
\end{theorem}
\begin{proof}
We denoted $\hat{\bz} = \calA^{\rm att}(D, f)$. Because $\hat{\bz}$ is a post-function of $f$, $\hat{\bz}$ is also $(\varepsilon, \delta)$-differentially private.
For each $i=1, \cdots, n$,\\
\resizebox{\linewidth}{!}{
  \begin{minipage}{\linewidth}
     \begin{align}
     \label{equ:total_expectation_dp}
        \bbE [g(\hat{\bz}_i, \bz_i) | \bz_{-i}] &= \bbE_{\bz_i}\bbE_{\hat{\bz}_i|\bz_{-i}, \bz_i} [g(\hat{\bz}_i, \bz_i) ]\nonumber\\
        &=\bbE_{\bz_i}\bbE_{\hat{\bz}_i|\bz_{-i}, \bz_i} [g(\hat{\bz}_i, \bz_i) - 1] + 1.
        % &\leq e^{-\varepsilon}  `\bbE_{\bz_i|X}\bbE_{\hat{\bz}_i|\bz_{-i}, \bz_i=z^*} [g(\hat{\bz}_i, \bz_i) - 1] + 1
    \end{align}
  \end{minipage}
}
By following the definition of label differential privacy, when $\calZ$ is a continuous space, we have\\
\resizebox{\linewidth}{!}{
  \begin{minipage}{\linewidth}
     \begin{align*}
        &\bbE_{\hat{\bz}_i|\bz_{-i}, \bz_i} [g(\hat{\bz}_i, \bz_i) - 1]\\
        &=\int_{z\in\calZ}\bbP(\hat{\bz}_i=z|\bz_{-i}, \bz_i)\cdot(g(\hat{\bz}_i, \bz_i) - 1) \diff z\\
        &\leq \int_{z\in\calZ}e^{-\varepsilon}\left(\bbP(\hat{\bz}_i=z|\bz_{-i},  \bz_i={\color{blue} z^*}) -\delta \right) (g(\hat{\bz}_i, \bz_i) - 1)\diff z\\
        % & -\int_{z\in\calZ} e^{-\varepsilon}\cdot \delta\cdot(g(\hat{\bz}_i, \bz_i) - 1)\\
        &= e^{-\varepsilon} \bbE_{\hat{\bz}_i|\bz_{-i}, \bz_i={\color{blue}z^*}} [g(\hat{\bz}_i, \bz_i)] - e^{-\varepsilon} +  e^{-\varepsilon}\delta \int_{z\in\calZ} (1 - g(\hat{\bz}_i, \bz_i) )\\
        &\leq e^{-\varepsilon} \bbE_{\hat{\bz}_i|\bz_{-i}, \bz_i={\color{blue}z^*}} [g(\hat{\bz}_i, \bz_i)] - e^{-\varepsilon} +  e^{-\varepsilon}\delta|\calZ|\\
        &\leq e^{-\varepsilon} \bbE_{\hat{\bz}_i|\bz_{-i}, \bz_i={\color{blue}z^*}} [g(\hat{\bz}_i, \bz_i)] - e^{-\varepsilon} +  \delta|\calZ|
        % &\leq e^{-\varepsilon} \max_{y\in \calY} [g(y, \bz_i)] - e^{-\varepsilon} +  e^{-\varepsilon}\cdot \delta \cdot|\calZ|\\
        % &\leq e^{-\varepsilon}  `\bbE_{\bz_i|X}\bbE_{\hat{\bz}_i|\bz_{-i}, \bz_i=z^*} [g(\hat{\bz}_i, \bz_i) - 1] + 1
    \end{align*}
  \end{minipage}
}
where ${\color{blue}z^*}$ is any fixed label in $\calZ$, $|\calZ|:=\int_{z\in\calZ} 1\diff z$. . It is similar when $\calZ$ is discrete: the above bound still holds by replacing integral operators and probability density function with summation operators and probability mass function and $|\calZ|$ is the size of $\calZ$.

Therefore, by plugging the above inequality into \autoref{equ:total_expectation_dp} we have\\
\resizebox{\linewidth}{!}{
  \begin{minipage}{\linewidth}
\begin{align*}
&\bbE [g(\hat{\bz}_i, \bz_i) | \bz_{-i}] \\
&=\bbE_{\bz_i}\bbE_{\hat{\bz}_i|\bz_{-i}, \bz_i} [g(\hat{\bz}_i, \bz_i)-1] + 1\\
&\leq \bbE_{\bz_i}\left[e^{-\varepsilon} \bbE_{\hat{\bz}_i|\bz_{-i}, \bz_i={z^*}} [g(\hat{\bz}_i, \bz_i)] - e^{-\varepsilon} +  \delta|\calZ| + 1\right]\\
&=e^{-\varepsilon}\bbE_{\bz_i}\bbE_{\hat{\bz}_i|\bz_{-i}, \bz_i={z^*}}[g(\hat{\bz}_i, \bz_i)] - e^{-\varepsilon} + \delta|\calZ|\\
&=e^{-\varepsilon}\bbE_{\hat{\bz}_i|\bz_{-i}, \bz_i={z^*}}\bbE_{\bz_i}[g(\hat{\bz}_i, \bz_i)] - e^{-\varepsilon} +  \delta|\calZ| + 1\\
&\leq e^{-\varepsilon}\max_{z\in\calZ} \bbE_{\bz_i}[g(z, \bz_i)] - e^{-\varepsilon} + \delta|\calZ| + 1.
\end{align*}
  \end{minipage}
}
Finally, we could derive the bound for the excess advantage ${\rm \text{Exc-Adv}}\left(\calA^{\rm att}, \calK\right)$:\\
\resizebox{\linewidth}{!}{
  \begin{minipage}{\linewidth}
\begin{align*}
 &{\rm \text{Adv}}\left(\calA^{\rm att}, \calK\right) 
    - \max_{z\in\calZ} \bbE_{\bz_i}[g(z, \bz_i)]\\
 &=\bbE [g(\hat{\bz}_i, \bz_i)] - \max_{z\in\calZ} \bbE_{\bz_i}[g(z, \bz_i)]\\
 &=\bbE_{\bz_{-i}}\bbE [g(\hat{\bz}_i, \bz_i) | \bz_{-i}] - \max_{z\in\calZ} \bbE_{\bz_i}[g(z, \bz_i)]\\
 &\leq \left(e^{-\varepsilon}-1\right)\max_{z\in\calZ} \bbE_{\bz_i}[g(z, \bz_i)] - e^{-\varepsilon} +  \delta|\calZ| + 1\\
 &\leq 1 - e^{-\varepsilon} + \delta |\calZ|.
\end{align*}
  \end{minipage}
}
\end{proof}
